# Supplementary material for: LLaVA-Grounding: Grounded Visual Chat with Large Multimodal Models
Source: arXiv:2312.02949 source file (2023-12-05)
Supplement: Supplementary file 1 [file vis_supp.tex]

\begin{figure*}[t!]
\centering  
\vspace{-0mm}
\includegraphics[width=0.99\textwidth]{images/src/vis_supp.pdf} \\
% \vspace{-2mm}
\caption{Comparison of our method with other LMMs in grounded description.\hao{large font}\hao{best prompt for each method.}}
\label{fig:visualization supp}  
% \caption{}
  % \vspace{-5mm}
\end{figure*}
