# Supplementary material for: LLaVA-Grounding: Grounded Visual Chat with Large Multimodal Models
Source: arXiv:2312.02949 source file (2023-12-05)
Supplement: Supplementary file 2 [file vis_supp_vp.tex]

\begin{figure*}[t!]
\centering  
\vspace{-0mm}
\includegraphics[width=0.99\textwidth]{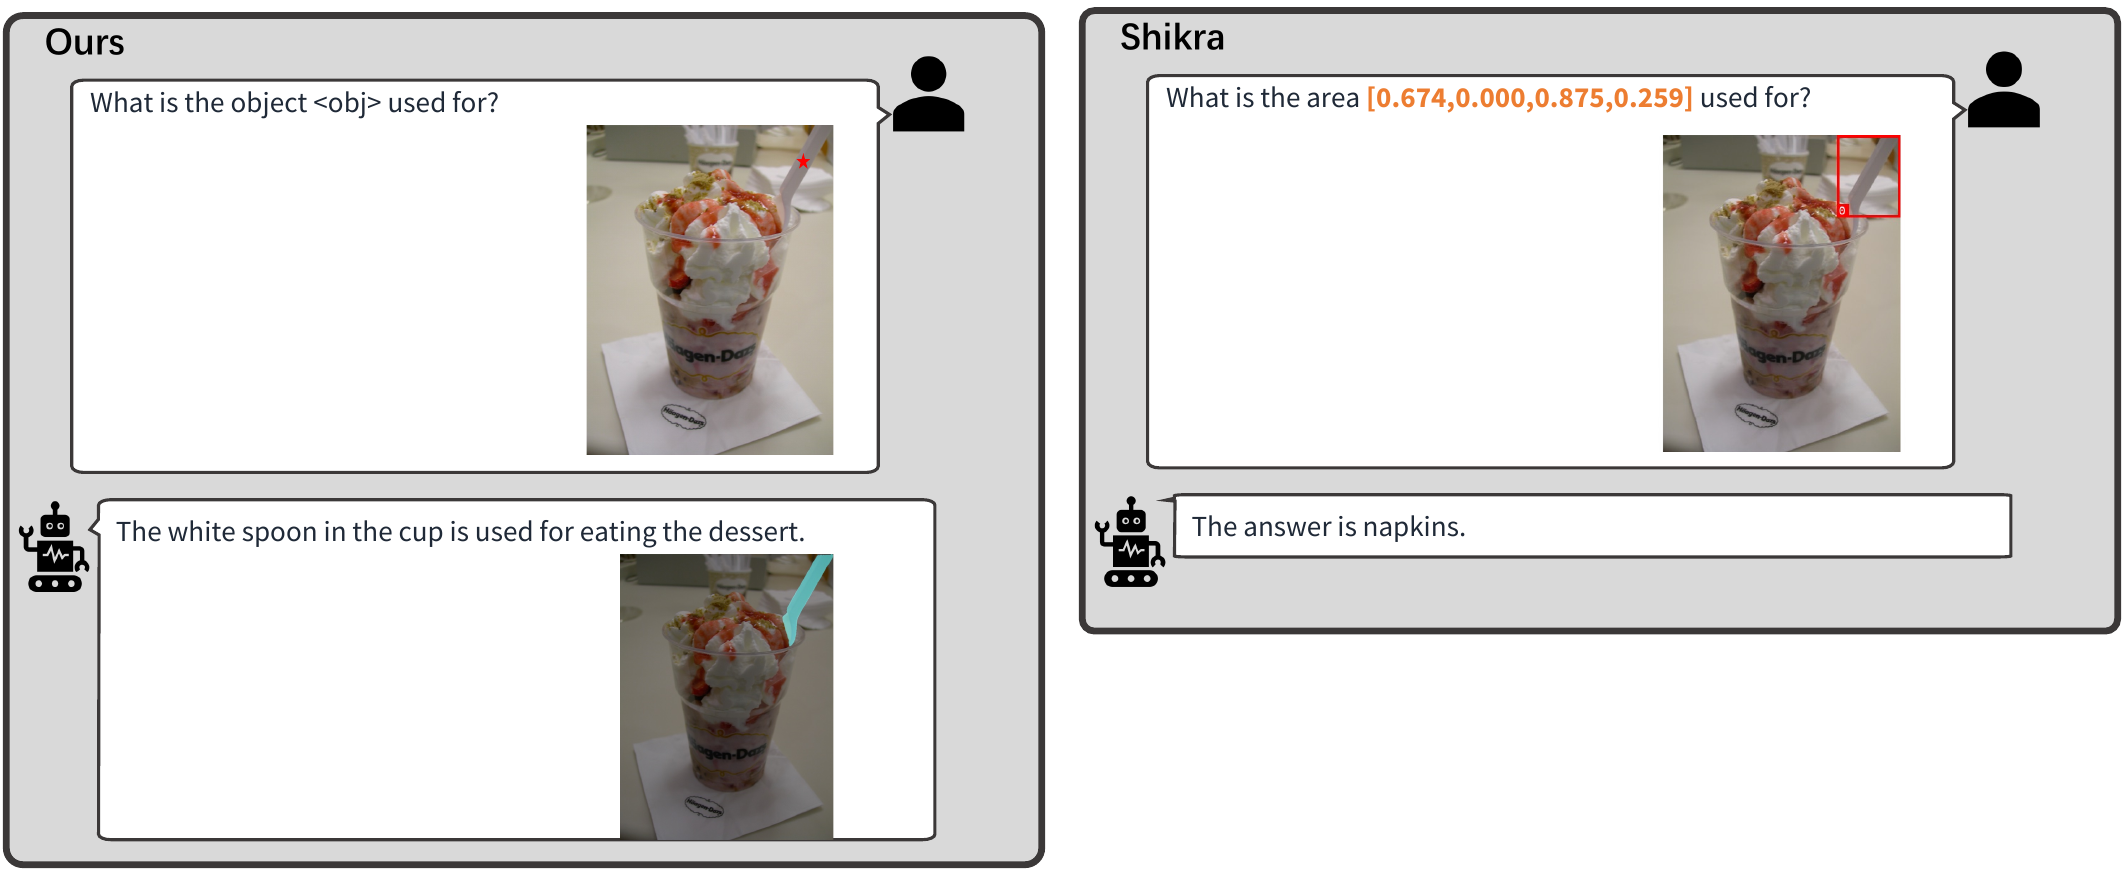} \\
% \vspace{-2mm}
\caption{Comparison of our method with Shikra in visual prompts. In the left block, the red star is user's click and the highlight region in response is the predicted mask from the prompt encoder. In the right block, the red box is drawn by the user. }
\label{fig:visualization supp vp}  
% \caption{}
  % \vspace{-5mm}
\end{figure*}
